# Supplementary material for: Introducing emotions in the reasoning cycle ofnormative aware agents
Source: arXiv:2209.10049 source file (2022-09-21)
Supplement: Supplementary file 1 [file appendix.tex]

% POR SI EN ALGÚN MOMENTO ES ÚTIL %

\begin{algorithm}
\caption{Prohibition norm acquisition}\label{alg:prohibition_acquisition}
\SetKwFunction{AddPlan}{.add\_plan}
\SetKwComment{Comment}{$\triangleright$ }{}
\KwIn{Norm=$prohibition(Action, Parameters)$}
\KwOut{new plans to enable norm compliance added to plan list}

add belief $prohibition(Action, Parameters)$\;
acquire list $relevantPlansAffected$ \Comment*[r]{Check Algorithm \ref{alg:relevant_plans_modification}}
refine $relevantPlansAffected$ \Comment*[r]{Check Algorithm \ref{alg:relevant_plans_refinement}}
remove the relevant plans from the plan list\;
create list $normativePlans$ \Comment*[r]{Check Algorithm \ref{alg:create_new_normative_plans}}
\lForEach{plan $p$ on $normativePlans$}{\AddPlan{p}}
\end{algorithm}

\begin{algorithm}
\caption{Relevant plans acquisition and modification (Java)}\label{alg:relevant_plans_modification}
\SetKwFunction{RelevantPlans}{.relevant\_plans}
\KwData{$Action$ and list of $Parameters$}
\KwResult{Jason Trigger with format similar to $Action(\_)$ usable with the \RelevantPlans internal action}
\eIf{$Parameters$ is atomic}{
    $terms$ = '\_'\;
}{\If{$Parameters$ is List}{
    \lForEach{Parameter $p$ on $Parameters$}{$terms$ += '\_'}
 }
}
return trigger $Action$($terms$)\;
\end{algorithm}

\begin{algorithm}
\caption{Relevant plan list refinement using Parameters (Java)}\label{alg:relevant_plans_refinement}
\KwData{$planList$ as args[0], $labelList$ as args[1], $parameters$ as args[2]}
\KwResult{$planList$ and $labelList$ with plans and labels that contains $parameters$}
\ForEach{plan p on $planList$}{
    \If{$p$ contains $parameters$}{
        $planList$.remove($p$)\;
        $labelList$.remove($p$)\;
    }
}
return $planList$, $labelList$\;
\end{algorithm}

\begin{algorithm}
\caption{Prohibition plan creation (Java)}\label{alg:create_new_normative_plans}
\KwData{$planList$ as args[0]}
\KwResult{$planList$ with new normative aware prohibition plans}
\SetKwComment{Comment}{// }{ }
\ForEach{plan $p$ on $planList$}{
    pattern = ``(\_[0-9]*)"\;
    i = 1\;
    stringNewTerms = ``"\;
    HashMap$<$Term, Term$>$ newTerms = new HashMap$<>$();
    \Comment{If the plan is generic it might contain anonymous variables, representend by an underscore in Jason. We need to replace them with a new variable with a workable syntax}
    \ForEach{$term$ in $p$}{
        \eIf{$pattern$ matches $term$}{
            newTerms.put($pattern$, new StringTermImpl(``Param"+i))\;
            stringNewTerms += ``Param"+i\;
            i++\;
        }{
            stringNewTerms += $t$\;
        }
    }
    triggerAction = $plan$.name \Comment*[l]{$plan$ functor}
    newTrigger = new Trigger(TEOperator.add, TEType.achieve, triggerAction+stringNewTerms) \Comment*[l]{The header of the new plans}
}
\end{algorithm}

{
\setlength{\interspacetitleruled}{-.4pt}%
\begin{algorithm}
\setcounter{AlgoLine}{12}
\SetKwComment{Comment}{// }{ }
%This is to hide Begin keyword
\SetKwBlock{Begin}{}{end} 
\TitleOfAlgo{Continuation (1) of Algorithm \ref{alg:create_new_normative_plans}}
\Begin{
    \Comment{1. Modify the original plan to point that it should work if the prohibition is not established, i.e. the action is allowed}
	\Comment{1.1. Create the new label}
	annots.add(``normative")\;
	annots.add(``not\_prohibition")\;
	newLabel.addAnnots(annots)\;
	\Comment{1.2 Create the new logical formula}
	planContext = plan.getContext()\;
	String triggerTerms = stringNewTerms.values().toString().replace("\"", "")\;
    \eIf{planContext == null}
    {
    	newContext = ``not prohibition("+triggerAction+``, " + triggerTerms + ``)"\;
    }
    {
    	newContext = planContext.toString() + `` \& not prohibition("+triggerAction+``, " + triggerTerms + ")"\;
    }
	newLogicalFormula = newContext\;
	\Comment{1.3. Loop over the new body and update it back properly using the HashMap}
	newPlanBody = ``"\;
	\While{planBody.getBodyNext() != null}{
	    Check if the line contains a word stored in $newTerms$ and replace it \;
	    planBody = planBody.getBodyNext();
    }
	\Comment{1.4. Form final plan}
	Plan notProhibitionPlan = new Plan(newLabel, newTrigger, newLogicalFormula, planBody)\;     
}
\end{algorithm}
}

{
\setlength{\interspacetitleruled}{-.4pt}%
\begin{algorithm}
\setcounter{AlgoLine}{27}
\SetKwComment{Comment}{// }{ }
%This is to hide Begin keyword
\SetKwBlock{Begin}{}{end} 
\TitleOfAlgo{Continuation (2) of Algorithm \ref{alg:create_new_normative_plans}}
\Begin{
    \Comment{2. Insert the new plan}
    \Comment{2.1}
    \Comment{2.2}
    \Comment{2.3}
    \Comment{3. }
    
    // 2. Insert the new plan
	// 2.1.
	String namespace2 = planLabel.getFunctor() + "2";
	ListTerm annots2 = planLabel.getAnnots().cloneLT();
	Atom aNormative2 = new Atom("normative");
	Atom aProhibition2 = new Atom("prohibition");
	annots2.add(aNormative2);
	annots2.add(aProhibition2);
	newLabel = new Pred(namespace2);
	newLabel.addAnnots(annots2);

	// 2.2.
	//triggerTerms = "[Param1]";
	if (planContext == null)
		newContext = "prohibition(publish, " + triggerTerms + ")";
	else
		newContext = planContext.toString() + " \& prohibition(publish, " + triggerTerms + ")";
	newLogicalFormula = LogExpr.parseExpr(newContext);

	// 2.3.
	// Term t = new Structure(".print(\"I cannot do this action\")");
	PlanBody newEmptyBody = new PlanBodyImpl(BodyType.none);
	//TODO: Cambiar t por planTrigger
	Plan prohibitionPlan = new Plan(newLabel, newTrigger, newLogicalFormula, newEmptyBody);

	// 3. We add the new plans to the results
	resultList.add(notProhibitionPlan);
	resultList.add(prohibitionPlan);
}
\end{algorithm}
}
